# Supplementary material for: Modelling electroweak physics for the forward region
Source: arXiv:1608.06906 source file (2016-08-30)
Supplement: Supplementary file 1 [file appendix.tex]

\clearpage

{\noindent\bf\Large Appendices}

\appendix

Test.
